# Supplementary material for: Asymmetric cloning in quantum information theory
Source: arXiv:2309.17229 source file (2023-09-29)
Supplement: Supplementary file 1 [file appendixB.tex]

\chapter{Résumé en français}

Cette annexe est dédiée à un résumé détaillé de la thèse, en français, conformément au code français de l'éducation article L121-3.

\section{Introduction}

La théorie de l'information quantique est un domaine interdisciplinaire qui combine les principes de la mécanique quantique et de la théorie de l'information, reliant ainsi la physique théorique, l'informatique et les mathématiques. L'objectif principal de ce domaine de recherche est de comprendre les propriétés quantiques des systèmes physiques, afin de pouvoir les manipuler et les transmettre de manière efficace. En tant que domaine de recherche en évolution rapide, la théorie de l'information quantique a le potentiel de catalyser des avancées significatives en matière de cryptographie, de calcul et de communication.

Un concept fondamental de la théorie de l'information quantique est l'intrication quantique, qui fait référence aux corrélations qui existent entre deux ou plusieurs systèmes quantiques. Ces corrélations non-classiques permettent de réaliser des tâches qui sont impossibles dans les systèmes classiques. L'intrication quantique est devenue une ressource clé pour le traitement de l'information quantique, permettant des opérations telles que la téléportation quantique, le codage superdense et la correction d'erreurs quantiques.

Les canaux quantiques, un autre concept clé de la théorie de l'information quantique, décrivent la transmission d'informations quantiques. Le développement de techniques efficaces et fiables pour la transmission d'informations quantiques est essentiel pour la réalisation de la communication quantique et de l'informatique quantique. Les canaux de clonage quantiques, une catégorie spécifique de canaux quantiques, font référence à la notion de clonage quantique, qui implique la création de plusieurs copies identiques d'un état quantique inconnu. Bien que le clonage quantique parfait soit impossible, pour un état quantique inconnu, en raison du théorème de non-clonage, résultant de la linéarité de la mécanique quantique, la création de copies approximatives reste réalisable.

En outre, il est important de souligner que la théorie de l'information quantique étend la théorie de l'information classique en incluant les propriétés uniques de mécanique quantique. En effet, les systèmes quantiques peuvent être utilisés pour stocker et manipuler de l'information classique.

Cette thèse vise à fournir une investigation exhaustive des problèmes de clonage quantique, ainsi que des problèmes d'intrication quantique associés. L'analyse de ces sujets est basée sur l'application des concepts de base de la théorie de la représentation, en particulier ceux associés au groupe symétrique. L'utilisation de ces concepts permet l'unification de différents sujets et une compréhension plus étendue des questions traitées.

Pour atteindre cet objectif, l'exploration initiale de cette thèse implique la notion fondamentale de dualité Schur-Weyl, qui fournit un lien critique entre le groupe symétrique et le groupe unitaire. Cette dualité permet une représentation et une manipulation efficaces des systèmes quantiques, en faisant ainsi un outil précieux pour la recherche en théorie de l'information quantique. De plus, différentes extensions de la dualité Schur-Weyl, impliquant d'autres groupes et algèbres, sont étudiées dans cette thèse.

Une application principale de la dualité Schur-Weyl qui reçoit une attention particulière est le clonage quantique, qui implique la création de plusieurs copies d'un état quantique inconnu. Le cas $1 \to 2$ et le cas plus général $1 \to N$, où $N$ copies d'un état inconnu sont créées, sont étudiés dans cette thèse, fournissant de nouvelles perspectives sur les contraintes imposées par le théorème de non-clonage.

L'investigation de cette thèse se poursuit ensuite avec un problème d'intrication quantique plus général, en explorant sa relation avec la dualité Schur-Weyl et en développant de nouvelles techniques pour analyser et résoudre le problème.

La contribution principale de cette thèse est l'application de la théorie de la représentation à des problèmes clés de la théorie de l'information quantique, en particulier ceux liés aux limites du clonage quantique et à l'intrication quantique.

\section{Théorie de l'information quantique}

Soit $\emph{\mathcal{H}} \coloneqq \mathbb{C}^d$ un espace de Hilbert complexe fini de dimension $d$, et $\emph{\mathcal{M}_d}$ l'espace des matrices complexes $d \times d$ agissant sur $\mathcal{H}$. Étant donné une matrice $M \in \mathcal{M}_d$, sa transposée conjuguée ${\bar{M}}^\T$ est notée $\emph{M^*}$. Le produit intérieur de Frobenius $\emph{\scalar{\cdot}{\cdot}}$ sur $\mathcal{M}_d$ est défini par,
\begin{equation*}
    \scalar{A}{B} \coloneqq \Tr \1[ A^* B \1].
\end{equation*}

En utilisant la notation de Dirac, les vecteurs sont représentés par des kets, notés $\emph{\ket{\psi}}$, tandis que leurs duaux sont appelés bras, notés $\emph{\bra{\psi}}$. Le produit intérieur sur $\mathcal{H}$ devient simplement,
\begin{equation*}
    \braket{\psi}{\phi} \in \mathbb{C},
\end{equation*}
et le produit extérieur,
\begin{equation*}
    \ketbra{\psi}{\phi} \in \mathcal{M}_d.
\end{equation*}
La \emph{base de calcul} de $\mathcal{H}$ est définie par: $\ket{0}, \ldots, \ket{d-1}$.

Sur un produit tensoriel $\mathcal{H}_1 \otimes \cdots \otimes \mathcal{H}_n$, les notations $\emph{M_{(i)}}$ et $\emph{v_{(i)}}$ pour une matrice $M \in \mathcal{M}_{d_i}$ et un vecteur $v \in \mathcal{H}_i$ sont utilisées pour désigner la position de la matrice et du vecteur sur l'espace tensoriel $\mathcal{H}_i$. Étant donné une matrice $M \in \mathcal{M}_{d_1} \otimes \cdots \otimes \mathcal{M}_{d_n}$, la transposée partielle $\emph{M^\Tpartial}$ désigne l'opération de transposition sur premier tenseur $\mathcal{H}_1$, et la trace partielle $\emph{\Tr_i [M]}$ désigne l'opération de trace sur le tenseur $\mathcal{H}_i$.

De plus, la notation $\emph{[n]}$ est utilisée pour désigner alternativement l'ensemble $\{1, \ldots, n\}$ ou l'ensemble $\{0, 1, \ldots, n\}$. Les deux utilisations sont non ambiguës dans leur contexte. 

L'ensemble des \emph{états quantiques} sur le \emph{système quantique} $\mathcal{H}$ est défini par l'ensemble convexe:
\begin{equation*}
    \emph{\mathcal{D}_d} \coloneqq \set{\rho \in \mathcal{M}_d}{\Tr \rho = 1 \text{ and } \rho \geq 0}.
\end{equation*}
Un point extrémal de $\mathcal{D}_d$ est appelé un \emph{état quantique pur}, et est un projecteur de rang $1$ sur un vecteur $\ket{\psi} \in \mathcal{H}$. Un \emph{état quantique mixte} est donc une combinaison convexe d'états quantiques purs. L'état quantique le plus central de $\mathcal{D}_d$ est appelé l'état \emph{maximalement mixte}, et est $\emph{\mathrm{I}} \coloneqq \frac{I_d}{d}$.

Un \emph{système quantique composé} est un produit tensoriel de systèmes quantiques $\mathcal{H}_1 \otimes \cdots \otimes \mathcal{H}_n$. Dans un système quantique composé biparti $\mathcal{H}_A \otimes \mathcal{H}_B$, un état quantique pur est un projecteur de rang $1$ vers un vecteur $\ket{\psi}_{(AB)} \in \mathcal{H}_A \otimes \mathcal{H}_B$. Si ce vecteur $\ket{\psi}_{(AB)}$ se décompose en
\begin{equation*}
    \ket{\psi}_{(AB)} = \ket{\psi}_A \otimes \ket{\psi}_B,
\end{equation*}
avec $\ket{\psi}_A$ et $\ket{\psi}_B$, les \emph{états quantiques réduits} sur $\mathcal{H}_A$ et $\mathcal{H}_B$ respectivement, alors l'état quantique pur est dit \emph{séparable}. Sinon l'état quantique pur est dit \emph{intriqué}. Un état quantique pur le plus intriqué sur $\mathcal{H} \otimes \mathcal{H}$ est appelé état \emph{maximalement intriqué}, et est le projecteur de rang $1$ $\emph{\omega} \coloneqq \ketbra{\Omega}{\Omega}$. Sur la base de calcul de $\mathcal{H}$, le vecteur $\emph{\ket{\Omega}}$ s'écrit
\begin{equation*}
    \ket{\Omega} \coloneqq \frac{1}{\sqrt{d}} \sum^{d-1}_{i=0} \ket{ii}.
\end{equation*}

Un état quantique $\rho$, combinaision convexe de l'état maximalement intriqué et de l'état maximalement mixte, est appelé \emph{état isotropique}:
\begin{align*}
    \rho &= \lambda \cdot \omega + (1 - \lambda) \mathrm{I}, & \lambda &\in [0, 1].
\end{align*}

La transformation la plus générale d'un état quantique, pur ou mixte, est appelée un \emph{canal quantique}, et est définie comme une application linéaire complètement positive et préservant la trace, i.e. un canal quantique est une application linéaire $\Phi : \mathcal{M}_d \to \mathcal{M}_{d^\prime}$ telle que $\Tr \1[ \Phi(X) \1] = \Tr \1[ X \1]$ pour tous $X \in \mathcal{M}_d$, et si $X \geq 0$ alors $\1( \Phi \otimes \id_D \1)(X) \geq 0$ pour tous $D \in \mathbb{N}$.

À toute application linéaire $\Phi : \mathcal{M}_d \to \mathcal{M}_{d^\prime}$ est associé une matrice $\emph{C_\Phi} \in \mathcal{M}_{d \times d^\prime}$ appelée \emph{matrice de Choi}, et définie par
\begin{align*}
    C_\Phi &\coloneqq (\id_d \otimes \Phi) \3( \sum^d_{i,j = 1} \ketbra{ii}{jj} \3) \\
    &= (\id_d \otimes \Phi) (d \cdot \omega).
\end{align*}
Depuis la matrice de Choi $C_\Phi$, il est possible de retrouver l'application linéaire $\Phi$ grâce à la formule:
\begin{equation*}
    \Phi(X) = \Tr_d \1[ C_\Phi (X^\T \otimes I_{d^{\prime}}) \1].
\end{equation*}
En particulier, l'application linéaire $\Phi$ est complètement positive si et seulement si $C_\Phi \geq 0$, et préserve la trace si et seulement si $\Tr_{d^\prime} \1[ C_\Phi \1] = I_d$.

La \emph{fidélité quantique} est une mesure de proximité entre deux états quantiques $\rho$ pur, et $\sigma$ quelconque. Elle est définie comme la fonction symétrique $\emph{F}$ de $\mathcal{D}_d \times \mathcal{D}_d$ vers $[0,1]$ par,
\begin{equation*}
    F(\rho, \sigma) \coloneqq \Tr \1[ \rho \sigma \1],
\end{equation*}
avec la propriété: $F(\rho, \sigma) = 1 \Leftrightarrow \rho = \sigma$.

\section{Problème de clonage quantique}

Le problème connu sous le nom de \emph{problème de clonage quantique} vise à identifier un canal quantique $\Phi$ spécifique, appelé \emph{canal de clonage quantique}, qui transforme un état quantique pur d'\textit{entrée} sur un système quantique $\mathcal{H}$, vers un état quantique mixte de \textit{sortie} sur un système quantique composé $\mathcal{H}^{\otimes N}$; de sorte que les marginales de \textit{sortie} de $\Phi$ soient aussi proches que possible de l'état d'\textit{entrée}. Pour cela, un \emph{vecteur de direction} noté $\emph{a}$ satisfaisant $a \in [0,1]^N$ et $\sum^N{i=1}a_i = 1$ est introduit. Le problème de clonage quantique est défini comme le problème d'optimisation donné par,
\begin{equation*}
    \sup_{\substack{\Phi~\text{canal} \\ \text{quantique}}} \sum^N_{i = 1} a_i \cdot \operatornamewithlimits{\mathbb{E}}_{\rho~\text{pur}} \2[ F \1( \Phi_i(\rho), \rho \1) \2],
\end{equation*}
où la moyenne est prise par rapport à la mesure uniforme sur les états quantiques purs.

Il n'existe pas de canal quantique $\Phi: \mathcal{M}_d \to {\1( \mathcal{M}_d \1)}^{\otimes N}$ tel que pour toutes marginales $\Phi_i$ et pour tous états purs $\rho$
\begin{equation*}
    F\1( \Phi_i(\rho), \rho \1) = 1,
\end{equation*}
i.e. $\Phi_i(\rho) = \rho$. Cette impossibilité découle du caractère linéaire des canaux quantiques, en effet en fixant une base $\ketbra{i}{j}$ de $\mathcal{M}_d$, il est possible de définir le canal quantique $\Phi$ par :
\begin{equation*}
    \Phi \1( \ketbra{i}{j} \1) \coloneqq \ketbra{i}{j}^{\otimes 2}.
\end{equation*}
Le canal quantique $\Phi$ copie parfaitement les états quantiques purs, projecteurs de rang $1$ sur les élements de la base $\ketbra{i}{j}$, en deux copies. Mais tous les  autres états quantiques purs ne seront pas correctement copiés, e.g. soit l'état quantique pur $\rho \coloneqq \ketbra{\psi}{\psi}$ avec $\ket{\psi} \coloneqq \frac{1}{\sqrt{2}} \1( \ket{i} + \ket{j} \1)$ où $i,j \in \{0, \ldots, d-1\}$, alors
\begin{align*}
    \Phi(\rho) &= \frac{1}{2} \2( \Phi \1( \ketbra{i}{i} \1) + \Phi \1( \ketbra{i}{j} \1) + \Phi \1( \ketbra{j}{i} \1) + \Phi \1( \ketbra{j}{j} \1) \3) \\
    &\neq \ketbra{\psi}{\psi}^{\otimes 2}.
\end{align*}
Ce résultat est connu sous le nom du \emph{théorème de non clonage}. Le problème de clonage quantique consiste alors à trouver un canal quantique qui soit le meilleur pour copier les états quantique pur selon une certaine direction.

Pour tous canaux de clonage quantiques $\Phi$, en posant pour chaque marginal $\Phi_i$, 
\begin{equation*}
    f_i \coloneqq \operatornamewithlimits{\mathbb{E}}_{\rho~\text{pur}} F\1( \Phi_i(\rho), \rho \1),
\end{equation*}
il est possible de trouver un canal quantique $\Psi$ tel que pour tous états quantiques purs $\rho$, et toutes marginales $\Psi_i$,
\begin{equation*}
    \Psi_i(\rho) = p_i \cdot \rho + (1-p_i) \frac{I_d}{d},
\end{equation*}
où $p_i \in [0, 1]$, et tel que $p_i$ et $f_i$ soient reliés par :
\begin{align*}
    f_i &= p_i  + \frac{(1 - p_i)}{d} & p_i &= \frac{d f_i - 1}{d - 1}.
\end{align*}
Ainsi le problème de clonage quantique peut être caractérisé par l'ensemble :
\begin{equation*}
    \emph{\mathcal{R}_{N,d}} \coloneqq \set{p \in [0,1]^N}{\exists \Phi: \mathcal{M}_d \xrightarrow[\text{quantique}]{\text{canal}} {\1( \mathcal{M}_d \1)}^{\otimes N} \text{ t.q. } \Phi_i(\rho) = p_i \cdot \rho + (1 - p_i) \frac{I_d}{d}}.
\end{equation*}

La première partie de cette thèse concerne l'article \cite{nechita2021geometrical} sur le problème de clonage quantique $1 \to 2$. L'ensemble $\mathcal{R}_{2,d}$ est l'\emph{union d'ellipses} indexée par $\lambda \in [0, d]$:
\begin{equation*}
    \qquad \frac{x^2}{a^2_\lambda} + \frac{(y - c_\lambda)^2}{b^2_\lambda} \leq 1,
\end{equation*}
où $a_\lambda \coloneqq \frac{\lambda}{\sqrt{d^2 - 1}}, b_\lambda \coloneqq \frac{\lambda}{d^2 - 1}$ et $c_\lambda \coloneqq \frac{\lambda d - 2}{d^2 - 1}$. Les paramètres $x$ et $y$ peuvent être exprimés comme,
\begin{align*}
    x &=  p_1 - p_2 & y &=  p_1 + p_2.
\end{align*}

Les canaux de clonage quantique optimaux $\Phi$ pour le problème de clonage quantique correspondent à $\lambda = d$, et leurs matrices de Choi s'écrivent comme une combinaison linéaire complexe de $4$ matrices $A, B, C$ et $D$ :
\begin{equation*}
    C_\Phi = a \cdot A + b \cdot B + c \cdot C + d \cdot D,
\end{equation*}
tel que $a, b \in \mathbb{R}$ et,
\begin{align*}
    c &= \bar{d} & d (a + b) + 2 \Re(c) &= 1 & a b &\geq |c|^2.
\end{align*}

En général, un canal de clonage quantique $\Phi$, pas nécessairement optimale, a une matrice de Choi qui s'écrit comme une combinaison linéaire complexe de $6$ matrices $A, B, C, D, E$ et $F$ :
\begin{equation*}
    C_\Phi = a \cdot A + b \cdot B + c \cdot C + d \cdot D + e \cdot E + f \cdot F.
\end{equation*}
Ces $6$ matrices correspondent à des opérateurs de permutation des tenseurs de $\mathcal{H}^{\otimes 3}$, transposée partiellement sur le premier tenseur. Ainsi,
\begin{itemize}
    \item[$\bullet$] $A^\Tpartial$ est la transposition du premier et deuxième tenseur,
    \item[$\bullet$] $B^\Tpartial$ est la transposition du premier et troisième tenseur,
    \item[$\bullet$] $C^\Tpartial$ est le cycle décroissant des trois tenseurs,
    \item[$\bullet$] $D^\Tpartial$ est le cycle croissant des trois tenseurs,
    \item[$\bullet$] $E^\Tpartial$ est l'identité,
    \item[$\bullet$] $F^\Tpartial$ est la transposition du deuxième et troisième tenseur.
\end{itemize}

La deuxième partie de cette thèse concerne l'article \cite{nechita2022asymmetric} sur le problème de clonage quantique $1 \to N$. Le problème de clonage quantique peut être simplifié en utilisant,
\begin{align*}
    &\sum^N_{i = 1} a_i \cdot \operatornamewithlimits{\mathbb{E}}_{\rho~\text{pur}} \2[ F \1( \Phi_i(\rho), \rho \1) \2] \\
    &= \sum^N_{i = 1} a_i \cdot \operatornamewithlimits{\mathbb{E}}_{\rho~\text{pur}} \3[ \Tr \2[ \1( \Phi_i(\rho) \1) \rho \2] \3] \\
    &= \sum^N_{i = 1} a_i \cdot \operatornamewithlimits{\mathbb{E}}_{\rho~\text{pur}} \3[ \Tr \2[ \1( \Phi(\rho) \1) \1( \rho_{(i)} \otimes I^{\otimes (N-1)}_d \1) \2] \3] \\
    &= \sum^N_{i = 1} a_i \cdot \operatornamewithlimits{\mathbb{E}}_{\rho~\text{pur}} \3[ \Tr \2[ C_{\Phi} \1( \rho^\T_{(0)} \otimes \rho_{(i)} \otimes I^{\otimes (N-1)}_d \1) \2] \3] \\
    &= \sum^N_{i = 1} a_i \cdot \Tr \3[ C_{\Phi} \2( \operatornamewithlimits{\mathbb{E}}_{\rho~\text{pur}} \1[ \rho^\T_{(0)} \otimes \rho_{(i)} \1] \otimes I^{\otimes (N-1)}_d \2) \3] \\
    &= \frac{1}{d (d + 1)} \sum^N_{i = 1} a_i \cdot \Tr \3[ C_{\Phi} \2( \1( d^2 \cdot \mathrm{I}_{(0,i)} + d \cdot \omega_{(0,i)} \1) \otimes I^{\otimes (N-1)}_d \2) \3] \\
    &= \frac{1}{d (d + 1)} \Tr \4[ C_{\Phi} \3( \underbrace{\sum^N_{i = 1} a_i \cdot \1( d^2 \cdot \mathrm{I}_{(0,i)} + d \cdot \omega_{(0,i)} \1) \otimes I^{\otimes (N-1)}_d}_{R_a} \3) \4].
\end{align*}
Ce qui donne la borne supérieur sur le problème de clonage quantique dans la direction $a$ :
\begin{equation*}
    \sup_{\substack{\Phi~\text{canal} \\ \text{quantique}}} \sum^N_{i = 1} a_i \cdot \operatornamewithlimits{\mathbb{E}}_{\rho~\text{pur}} \2[ F \1( \Phi_i(\rho), \rho \1) \2] \leq \frac{\lambda_{\text{max}}(R_a)}{d + 1},
\end{equation*}
où $\lambda_{\text{max}}(R_a)$ est la plus grande valeur propre de $R_a$.

Cette borne est atteinte pour toutes direction $a$ par le canal de clonage quantique $\Phi^a_{\text{opt}}$ défini par,
\begin{align*}
    \Phi^a_{\text{opt}} (\rho) &\coloneqq P_a \1( \rho \otimes I^{\otimes (N-1)}_d \1) P^*_a & &\forall \rho~\text{pur},
\end{align*}
où $P_a$ est donné comme une combinaison linéaire positive des opérateurs de permutation des tenseurs de $\mathcal{H}^{\otimes N}$. 

L'ensemble $\mathcal{R}_{N,d}$ est la \emph{partie positive de la boule unité dual d'une norme} définie sur $x \in \mathbb{R}^N$ par,
\begin{equation*}
    \norm{x} \coloneqq \frac{d \lambda_{\text{max}}(S_x) - \norm{x}_1}{d^2 - 1},
\end{equation*}
où $S_x \coloneqq \sum^N_{i=1} |x_i| \cdot \1( d \cdot \omega_{(0,i)} \1) \otimes I^{\otimes (N-1)}_d$.

\section{Problème d'intrication quantique multiparti}

Le problème de clonage quantique consiste à trouver un canal quantique $\Phi$ tel que pour tous états quantiques purs $\rho$, et toutes marginales $\Phi_i$,
\begin{equation*}
    \Psi_i(\rho) = p_i \cdot \rho + (1-p_i) \frac{I_d}{d},
\end{equation*}
avec des $p_i$ aussi grand que possible. La matrice de Choi des marginales de $\Phi$ est alors proportionnelle à un état isotropique, i.e.
\begin{equation*}
    C_{\Psi_i} = d \1( p_i \cdot \omega + (1-p_i) \mathrm{I} \1).
\end{equation*}
Sous forme de matrice de Choi, le problème de clonage quantique consiste à trouver, à normalisation près, un état quantique $\rho \in \mathcal{H}^{\otimes (N+1)}$ le plus maximalement intriqué, entre un tenseur (l'\textit{entrée}), et tous les autres (la \textit{sortie}). Si tous les $p_i$ sont égaux, le problème de clonage quantique $1 \to N$ devient un problème d'\emph{optimisation semi-définie positive} :
\begin{align*}
    \max_{\rho,p} \quad & p \\
    \text{s.t.} \quad & \rho_{0,i} = d \1( p \cdot \omega + (1 - p) \mathrm{I} \1), & \forall i \in \{1, \ldots, N\} \\
    & C_\Phi \geq 0,
\end{align*}
où $\rho_{0,i}$ designe l'état quantique réduit $\Tr_{[N] \setminus \{0,i\}} \1[ \rho \1]$.

La troisème partie de cette thèse concerne l'article \cite{christandl2013extendibility} sur variante de ce problème qui consiste consiste à trouver un état quantique $\rho \in \mathcal{H}^{\otimes N}$ le plus maximalement intriqué entre chaque paire de tenseur. Ce problème d'optimisation semi-définie positive s'écrit :
\begin{align*}
    p(N, d) \coloneqq \max_{\rho,p} \quad & p \\
    \text{s.t.} \quad & \rho_{i,j} = d \1( p \cdot \omega + (1 - p) \mathrm{I} \1), & \forall i \neq j \in \{1, \ldots, N\} \\
    & C_\Phi \geq 0,
\end{align*}
La solution de ce problème dépend à la fois de $N$ et de $d$, ainsi que de la parité de $N$ et de $d$, et s'éxprime par l'équation,
\begin{equation*}
    p(N,d) =
    \begin{cases}
        \frac{1}{N + N \bmod 2 - 1} &\text{ si $d > N$ ou soit $d$ soit $N$ est pair} \\
        \min \1\{ \frac{2 d + 1}{2 d N + 1}, \frac{1}{N - 1} \1\} &\text{ si $N \geq d$ et à la fois $d$ et $N$ sont impair}.
    \end{cases}
\end{equation*}
Les premières valeurs de $p(N,d)$ sont résumées dans le tableau suivant (en \tikz{\draw[fill = gray!30!white] (0,0) rectangle (1.5ex,1.5ex);} les valeurs de $p(N,d)$ pour lesquelles les états isotropiques $\rho_{i,j}$ sont séparables):
\begin{center}
    \begin{NiceTabular}{c|cccccccc}[columns-width = 2em, cell-space-limits = 0.25em]
        \CodeBefore
            \rectanglecolor{gray!30!white}{2-3}{2-9}
            \rectanglecolor{gray!30!white}{3-5}{3-9}
            \rectanglecolor{gray!30!white}{4-5}{4-9}
            \rectanglecolor{gray!30!white}{5-7}{5-9}
            \rectanglecolor{gray!30!white}{6-7}{6-9}
            \rectanglecolor{gray!30!white}{7-9}{7-9}
            \rectanglecolor{gray!30!white}{7-9}{8-9}
        \Body
        \diagbox{$d$}{$N$} & 2 & 3 & 4 & 5 & 6 & 7 & 8 & 9 \\ \hline
        2 &	1 &	\nicefrac{1}{3}  & \nicefrac{1}{3} & \nicefrac{1}{5}   & \nicefrac{1}{5} & \nicefrac{1}{7}   & \nicefrac{1}{7} & \nicefrac{1}{9} \\
        3 &	1 &	\nicefrac{7}{19} & \nicefrac{1}{3} & \nicefrac{7}{31}  & \nicefrac{1}{5} & \nicefrac{7}{43}  & \nicefrac{1}{7}& \nicefrac{1}{8} \\
        4 &	1 &	\nicefrac{1}{3}  & \nicefrac{1}{3} & \nicefrac{1}{5}   & \nicefrac{1}{5} & \nicefrac{1}{7}   & \nicefrac{1}{7}& \nicefrac{1}{9} \\
        5 &	1 &	\nicefrac{1}{3}  & \nicefrac{1}{3} & \nicefrac{11}{51} & \nicefrac{1}{5} & \nicefrac{11}{71} & \nicefrac{1}{7}& \nicefrac{11}{91} \\
        6 &	1 &	\nicefrac{1}{3}  & \nicefrac{1}{3} & \nicefrac{1}{5}   & \nicefrac{1}{5} & \nicefrac{1}{7}   & \nicefrac{1}{7}& \nicefrac{1}{9} \\
        7 & 1 & \nicefrac{1}{3}  & \nicefrac{1}{3} & \nicefrac{1}{5}   & \nicefrac{1}{5} & \nicefrac{5}{33}  & \nicefrac{1}{7}& \nicefrac{15}{127} \\
        8 & 1 & \nicefrac{1}{3}  & \nicefrac{1}{3} & \nicefrac{1}{5}   & \nicefrac{1}{5} & \nicefrac{1}{7}   & \nicefrac{1}{7}& \nicefrac{1}{9} \\
        9 & 1 & \nicefrac{1}{3}  & \nicefrac{1}{3} & \nicefrac{1}{5}   & \nicefrac{1}{5} & \nicefrac{1}{7}   & \nicefrac{1}{7}& \nicefrac{19}{163} \\
    \end{NiceTabular}
\end{center}
